# Supplementary material for: Leveraging Large Language Models for Solving Rare MIP Challenges
Source: arXiv:2409.04464 source file (2024-09-18)
Supplement: Supplementary file 1 [file 9appendix.tex]

\newpage
\section{Appendix}

\subsection{Prompt template}
\label{sec:appendix:prompt}
\begin{tcolorbox}[colback=yellow!5!white, colframe=black!75!black, title=Prompt Template, breakable]

Your task is to find the optimal solution for a carpool dispatch problem. If you cannot find the optimal solution, you should try to return a better feasible solution. The background is as follows:\\

Rules for vehicle-order pair:
\begin{itemize}

\item Each order is for one user only.

\item Each car can accept up to two orders.

\item There are three possible scenarios:
    \begin{enumerate}
        
   \item  Two people simultaneously hail a ride within a certain time range and decide to share the ride. The car will pick up Person A first, then Person B, and drop off Person A first, followed by Person B.
   
   \item  A person willing to share a ride, Person A, is already in the car, and the car has started the trip. A new carpool request from Person B is received. The car will go from its current location to pick up Person B, drop off Person A, and finally drop off Person B.
   
  \item  A person takes a ride from start to finish without any carpooling.
       \end{enumerate}

\end{itemize}
The objective is to minimize the total Manhattan distance between vehicles and users, considering all segments of the vehicle paths:\\

\textcolor{red}{-- LaTex code for building car pooling MIP model --}\\

You are given x and y coordinates (which are transformed from latitude and longitude using the Mercator projection method) for every empty vehicle, one-person vehicle, and user. The format is as follows:\\

EMPTY VEHICLES: (0) (x0, y0), (1) (x1, y1) ... \# Use "\textbackslash n" if no vehicles.

ONE ORDER VEHICLES: (0) (x0, y0), (1) (x1, y1) ... \# Use "\textbackslash n" if no one-order vehicles.

USERS: (0) (x0, y0), (1) (x1, y1) ... \# Use "\textbackslash n" if no users.\\

After transforming the latitude and longitude into x and y, it's much easier to calculate the Manhattan distance between two places. The Manhattan distance between (x0, y0) and (x1, y1) = abs(x1-x0) + abs(y1-y0)\\

\textcolor{blue}{EMPTY VEHICLES: (0) (86.97, 35.86), (1) (85.23, 36.74), (2) (95.62, 28.43),} 

\textcolor{blue}{ONE ORDER VEHICLES: (0) (90.55, 35.17), (1) (101.43, 44.49), (2) (100.56, 44.77), }

\textcolor{blue}{USERS: (0) (90.33, 35.82), (1) (97.04, 41.87), (2) (100.91, 42.75),\\ }

Below are some previous solutions. You can derive the optimal solution straightforwardly or derive the intermediate feasible solution step by step.\\

The term "gap" refers to the difference between the best-known solution and the best possible solution (optimal solution) within a given tolerance. The smaller the gap, the better the feasible solution. The format of previous solutions is:\\

x: (EMPTY\_0, USER\_5) (EMPTY\_2, USER\_3)... \# Car whose index is 'EMPTY\_0' is assigned to user whose index is 'USER\_5', and so on.

y: (EMPTY\_1, USER\_1, USER\_0) (EMPTY\_3, USER\_10, USER\_9)... \# Car whose index is 'EMPTY\_1' picks up user whose index is 'USER\_1', then user whose index is 'USER\_0', and so on.

z: (ONE\_REQUEST\_0, USER\_6), (ONE\_REQUEST\_1, USER\_7)... \# Car whose index is 'ONE\_REQUEST\_0' with one existing passenger picks up user whose index is 'USER\_6', and so on.\\

The x line is "\textbackslash n" if no one is assigned to a car alone.

The y line is "\textbackslash n" if no two people are assigned to share a car.

The z line is "\textbackslash n" if no one is assigned to a car with one existing passenger.

\textcolor{orange}{one of solutions starts:\\}
\textcolor{orange}{x: (0, 1) (1, 0)\\}

\textcolor{orange}{z: (1, 2) \\}
\textcolor{orange}{gap: 1.0, objective value: 24.36}\\
\textcolor{orange}{one of solutions ends}\\
\textcolor{purple}{( ----more exemplars -------)}
\end{tcolorbox}

\subsection{The Method for Calculating Distance}
\label{sec:appendix:distance}
Considering the high computational cost and impracticality of using Dijkstra’s algorithm to calculate distances for each instance, we simplify the model by calculating Manhattan distances when formulating the MIP. However, in the simulation process, Dijkstra’s algorithm is employed to simulate vehicle movement.
